# Supplementary material for: Emerging long orbits and self-similar temporal sequences in classical oscillators
Source: arXiv:1701.06889 ancillary file (2017-01-24)
Supplement: Supplementary file 1 [file supplement_hmortmanns23012017.pdf]

# Supplementary Material

Darka Labavić and Hildegard Meyer-Ortmanns

Department of Physics and Earth Sciences, Jacobs University Bremen, P.O.Box 750561, D-28725 Bremen, Germany

## 1 Regular implementation of frequencies

For the regular implementation we generate frequencies according to a deterministic procedure which leads to the choice of Fig.1 in the main text. We generate $M < N$ different frequencies, where M depends on the lattice extensions $l_x$ in x-direction and $l_y$ in y-direction and the fact that we have a hexagonal geometry. They are determined by solving the equation

$$\frac{j - 0.5}{M} = \int_{-\infty}^{\tilde{\omega}_j} g(\tilde{\omega}) d\tilde{\omega} \tag{1}$$

for $\tilde{\omega}_j$ with $g(\tilde{\omega})$ given by the Gaussian distribution $g(\omega) = \frac{1}{\sqrt{2\pi\sigma^2}} e^{-(\omega-\mu)^2/(2\sigma^2)}$ with $\mu = 1$ and $j \in 1, ..., M$ with $M = n_x + n_y - 1$, and $n_x = (l_x + mod(l_x, 2))/2$, $n_y = (l_y + mod(l_y, 2))/2$, where $n_{x(y)}$ denotes the number of different frequencies in x(y)-direction, respectively. The resulting $M$ different values of $\tilde{\omega}_j$ are assigned to at most four out of the six neighbors of a site on the hexagonal grid according to the following rules:

for $i = 1, nx$

for $j = 1, ny$

$$\begin{aligned}
\omega_{i,j} &= \tilde{\omega}_{i+j-1} \\
\omega_{l_x+1-i,j} &= \tilde{\omega}_{i+j-1} \\
\omega_{i,l_y+1-j} &= \tilde{\omega}_{i+j-1} \\
\omega_{l_x+1-i,l_y+1-j} &= \tilde{\omega}_{i+j-1}.
\end{aligned}$$

The double loop will in some cases revisit some of the sites of the lattice, but the assignment is done only once at the beginning of the numerical integration, so we need not further optimize the algorithm. For example, for the $4 \times 4$ lattice of Fig.1 of the main text we have $n_x = 2$, $n_y = 2$, and $M = 3$. If we take $\mu = 1$, and $\sigma = 0.01$, we obtain $\tilde{\omega}_1 = 0.99032578$ (purple color in Fig. 1(b) in the main text), $\tilde{\omega}_2 = 1.0$ (green), and $\tilde{\omega}_3 = 1.00967422$ (red). Let us now choose $i = 2$ and $j = 1$, then, according to the upper algorithm we have

$$\begin{aligned}
\omega_{2,1} &= \tilde{\omega}_2 \\
\omega_{3,1} &= \tilde{\omega}_2 \\
\omega_{2,4} &= \tilde{\omega}_2 \\
\omega_{3,4} &= \tilde{\omega}_2.
\end{aligned}$$

This way we achieve a "concentric" gradient of natural frequencies about the largest values in the center of the grid, adapted to a hexagonal lattice. Our choice of regular frequency assignment is analogous to the one in [1]. In [1] it was shown that the difference between random and regular assignment can have an impact on scaling relations. (For positively all-to-all coupled Kuramoto oscillators it leads to different hyperscaling in the vicinity of the synchronization transition.)

[1] H. Hong, H. Chaté, L.-H. Tang, H. Park, Phys. E **92**, 022122 (2015).

## 2 Legend for the representation of phases on the unit circle

Circles represent oscillators on a $4 \times 4$ hexagonal lattice. We assign colors and sizes such that in the representation on the unit circle the state (phase) of every site is visible, even if the phases perfectly overlap. Additionally, every second site has a dashed edge to make it better distinguishable within gray scales. The same colors are used in the time evolution of the phases in Fig. 5 of the main text, and Fig. 4 of this supplementary material.

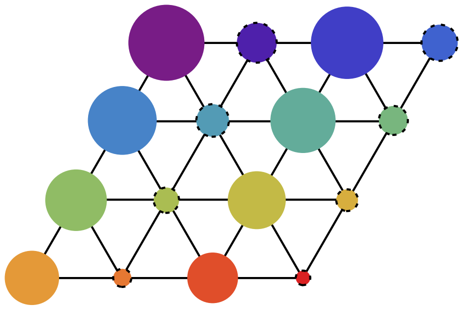

Figure 1: Legend for the representation of a temporary phase pattern on the unit circle.

## 3 Initial conditions $\phi_i(0)$ uniformly selected from $(0, 2\pi)$

The following two figures Fig. 2 and Fig. 3 show that long transients and long periods are not specific for the initial conditions from the vicinity of a fixed point in the phase differences at 0.5 for $\kappa > 0$, which is certainly far off from a stationary phase configuration at $\kappa < 0$. Also for a uniformly distributed selection from $(0, 2\pi)$ it seems unlikely to reach an attractor of the type of a heteroclinic orbit within a short transient time.

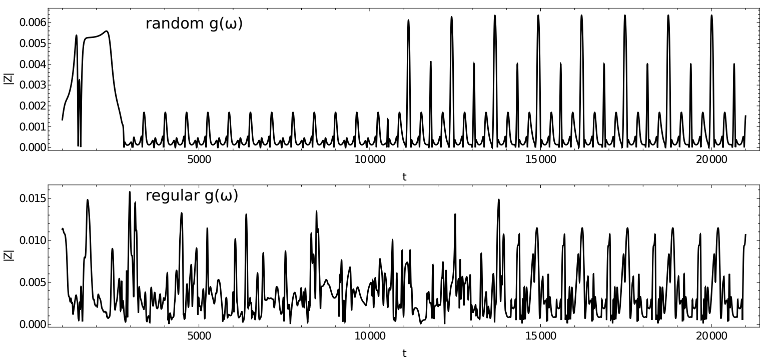


Figure 2: Transients of the order parameter with initial conditions from $\varphi_i \in (0, 2\pi)$ for random and regular assignment of natural frequencies for a $4 \times 4$ hexagonal lattice. The parameters are the same as in Fig.2 of the main text.

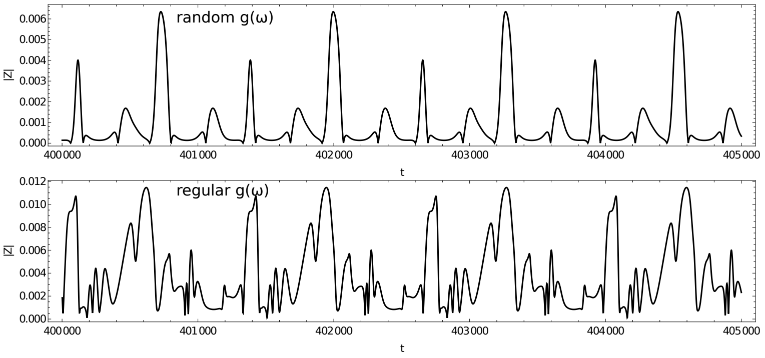


Figure 3: Periodic time evolution of the order parameter with initial conditions from $\varphi_i \in (0, 2\pi)$, for the same trajectories as of Fig. 2.

# 4 Zoom into the time evolution of individual phase trajectories

The following Fig. 4 illustrates the time evolution after a start in a temporary three-cluster state. Typical for this evolution is the change towards a different phase configuration after some time that can (or cannot) be characterized in terms of an n-cluster state. So it may come as a surprise that the phase patterns exactly repeat after a long cycle.

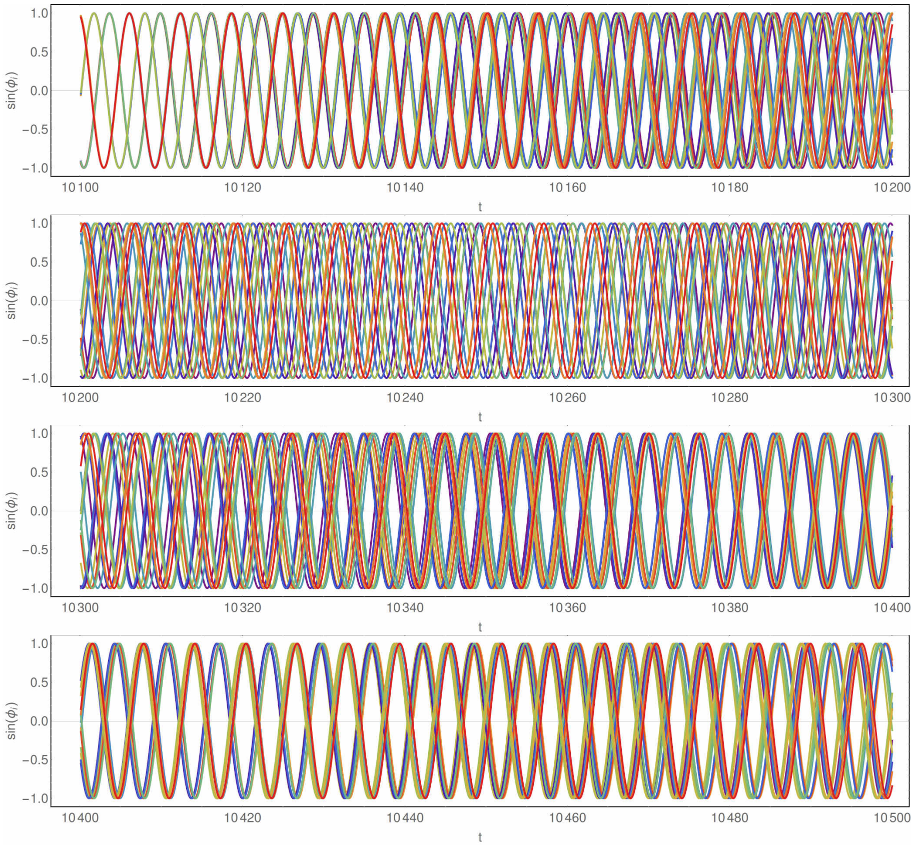


Figure 4: Time evolution of the phases, corresponding to the order parameter in Fig. 5 of the main text for 400 t.u. that corresponds to approximately one third of a long period. We show how the phases synchronize in different clusters starting with a three-cluster state (first red point in Fig. 5 of the main text). As the order parameter increases, clusters gradually spread reaching one of the maxima (second red point in Fig. 5 of the main text). When the next minimum is reached (at about 10420 t.u.), the system is in a two-cluster state. This kind of behavior goes on until the same three-cluster state is reached, and then the whole process repeats.

## 5 Long transient times and long periods

As we have seen in Fig.6 of the main text, long periods go along with long transients and scale with the inverse width of the regular frequency distributions. Additional remarks are in order how we determined the transient times. Transient times are determined in such a way that we first identify all peaks in one period of the order parameter, then we compare these peaks with peaks in the first 150000 t.u.. The first peak from the transient that coincides with one of the peaks from the period, defines our transient time. We eliminate the possibility of an accidental agreement by comparing the next available peak. An estimate of the error of this method is given by the largest time distance between two neighboring peaks in the order parameter, which, in general, is at most (happening in the case of only one peak per period) one period of the order parameter. This makes this kind of analysis involved, so we show the dependence of the time scales only for this range of $\sigma$.

## 6 Self-similar temporal sequences

As the following Fig. 5 shows, the self-similarity of the sequence of patterns of phase-locked motion holds for the whole range of widths between $\sigma = 0.001$ to $\sigma = 0.006$. Notice the different time scales of periods, ranging from $t = 50000$ for $\sigma = 0.001$ to $t = 8000$ for $\sigma = 0.006$. The ratio of any two periods t is almost exactly inversely proportional to the ratio of the corresponding widths $\sigma$ in the natural frequencies. For the displayed order parameter trajectories we find $\sigma t = 48.4 \pm 0.9$. We found similar self-similarity for other initial conditions.

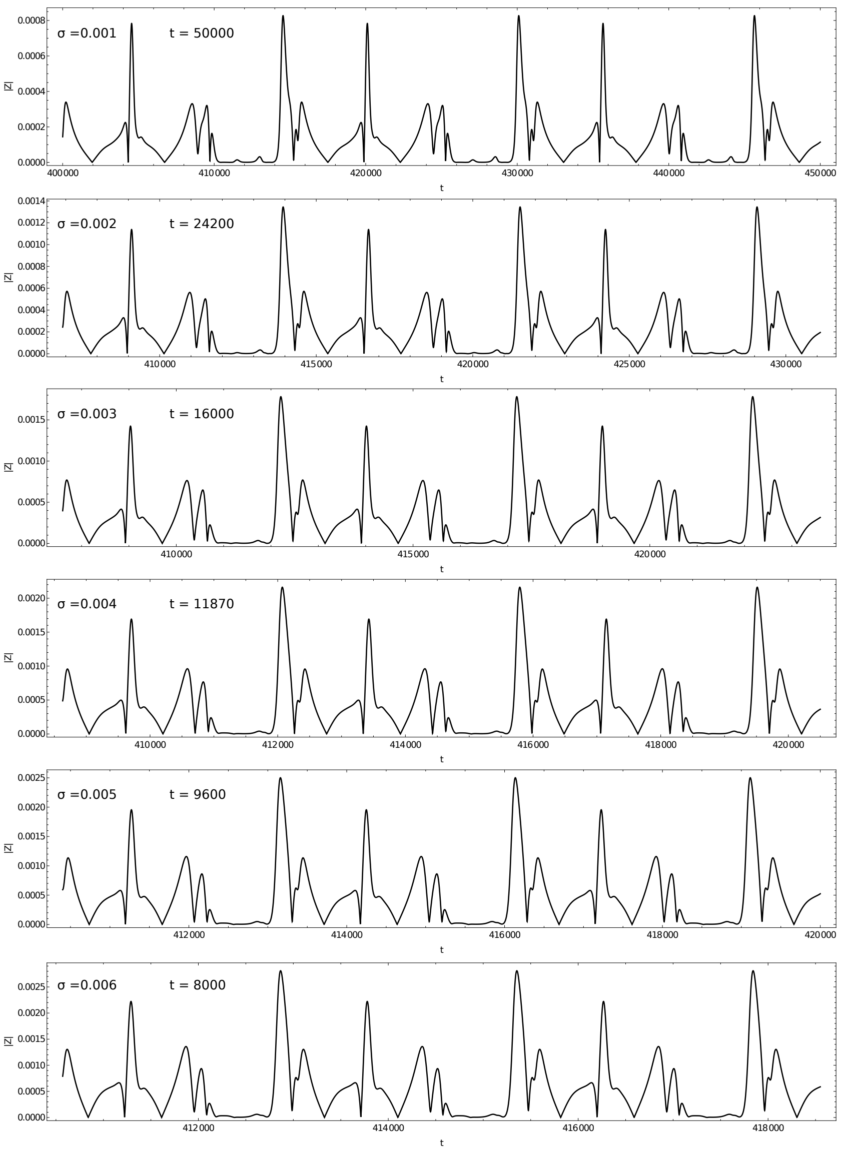


Figure 5: Self-similar trajectories of order parameters in time for six different widths of $g(\omega)$. The parameters are $\mu = 1$, $\kappa = -2$ on a $4x4$-grid for a fixed initial condition around the fixed point and regular frequency distribution.
